# Supplementary material for: An Overview of Catastrophic AI Risks
Source: arXiv:2306.12001 source file (2023-10-09)
Supplement: Supplementary file 1 [file 9-appendix.tex]

\section{Misconceptions}
Look at Yann's tweets for more misconceptions.
``This is a distraction from the real problems.''

\subsection{``AI risks are probably far in the future.''}
AI could cause catastrophic harm within years to decades if we don’t sufficiently manage its risks. Weaponized AI could be capable of killing large numbers of people in a matter of years. Some authoritarian regimes already use AI to control their populations. Many researchers think highly intelligent AI could be developed within the lifetimes of some people alive today.

\subsection{``AI risks are like other kinds of risks. We already know how to manage other kinds of risks.''}
AI poses some risks that are similar to those of existing technology as well as some that are unique to AI. In particular, AI’s ability to plan, deceive, replicate, coordinate and adapt, faster than humans, makes it a unique threat, especially as its intelligence increases. The threat is heightened if its goals do not align with humanity’s. Additionally, we do not know how to fully mitigate even traditional risks, as evidenced by ongoing accidents, misuse and unexpected behaviors of other technologies.

\subsection{``Enough people are already working to mitigate AI risks.''}
While the resources and number of people working on AI safety are growing, they are orders of magnitude smaller than the efforts to advance AI capabilities. While AI safety professionals have promising ideas for making AI safe, substantial uncertainty remains about the best paths forward. Having more people and resources would almost definitely help.

\subsection{``To pose a serious risk, AI must be sentient and evil.''}
An AI with powerful-but-narrow intelligence could still pose a threat, such as if it is in control of dangerous weapons. Powerful AI can pose serious risks even if it thinks it is doing what we want it to do, because it is very hard to account for the full range of human values and all the implicit assumptions that go into a set of instructions. Or, a human with malicious intentions could cause a powerful AI to perform catastrophic acts, even if the AI behaves exactly as instructed.

An AI with human-level intelligence or beyond might have a very different mind compared to ours, since it would be built in different ways from how our minds evolved. Sentience or consciousness isn't required for that mind to pose a catastrophic or existential risk. The risk comes from the AI’s ability to acquire power and resources and to have goals that don’t align with ours.


\subsection{``We'll always be able to stop or control AI, even if it starts to get out of hand.''}
Highly intelligent AI will be able to anticipate that we might want to stop it or control it, and it may evade our measures to contain it. Other humans might also have incentives to prevent us from stopping or controlling a particular AI. Coercive AI might even trick us that stopping or controlling it is not in our own best interest, until the AI has time to overpower us. Even AI that is trying to be helpful might prevent us from controlling it or turning it off, since being off would prevent it from helping us.


Dan notes:
``climate change is more pressing''
We are their creator
More benefits than harms
Humans program AI and can shut down AI if it becomes problematic

\section{Scenarios}
